# Supplementary material for: Improving Large-scale Paraphrase Acquisition and Generation
Source: arXiv:2210.03235 source file (2022-11-08)
Supplement: Supplementary file 1 [file data_details.tex]

\section{Paraphrase Generation Dataset Details}
All transformer-based models are finetuned with 32 batch size for 3 epochs on 4 Nivida A40 GPUs. Infersent and ESIM are trained on 1 GPU with 64/32 batch size. The epoch with highest precision on dev set are used for evaluation, as the models will be mainly used for extracting  paraphrase pairs from unlabeled data. 

\subsection{MultiPIT-New}
\label{sec:details:new}
We use trending topic and URL approaches that are introduced in section \ref{sec:dataset} to collect tweets from Oct 22nd 2021 to Dec 22nd 2021 and tweets from Jan 1st 2020 to Jun 31st 2021 respectively.
At first, we discard the trend topic and URL groups that have less than 6 sentences or 3 sentences respectively.
We rank sentences in each trend topic and URL group.
We pick top 5 sentences as seed sentences and top 6-55 sentences or the rest sentences, if the group has less than 55 sentences, as candidate sentences for trend topic group. Because in a group trend topic sentences are more diverse than URL sentences and there are more trend topic sentences than URL sentences, we pick top 2 sentences as seed sentences and top 3-42 sentences or the rest sentences, if the group has less than 42 sentences, as candidate sentences for URL group. Then we form pairs 
To examine how the model fine-tuned on MultiPIT performs on new data, we collect a test dataset that contains 400 new pairs of sentences that are annotated by an expert. Then we pair each seed sentence with all of the candidate sentences for each group. Finally, we use the identification model in Section \ref{sec:identification} to get the paraphrase pairs, which is \datasetname-New.

\subsection{MultiPIT-NMR}
\label{sec:details:nmr}
To get multiple paraphrases, we select groups that contain 

\subsection{Dataset Statistics}
\label{sec:details:statistics}

\input{fig/paraphrase_data_statistics}
