# Supplementary material for: Improving Large-scale Paraphrase Acquisition and Generation
Source: arXiv:2210.03235 source file (2022-11-08)
Supplement: Supplementary file 2 [file generation_setup_comparison_appendix.tex]

\begin{table*}[t]
\centering

\resizebox{\textwidth}{!}{
\begin{tabular}{@{}p{0.28\linewidth}l|rrrrrrr@{}}
\toprule
   \textbf{Data} & Size & BLEU-4 & ROUGE-L &\%new & \%eq & SELF-BLEU & BERT-Score & BERT-iBLEU  \\ 
   \midrule
   
     Multipit  & & \\
     \midrule
    M (BLEU $\leq 10$)    & \\
    M (BLEU $\leq 15$)    & \\
    M (BLEU $\leq 20$)    & \\
    M (BLEU $\leq 25$)    & \\
    \midrule
    M + New Trends    & \\
    M + New URL    & \\
    M + New Trends and URL& \\
    \midrule
    M + New Trends and URL (B-4 $\leq 10$ \& B-S $\geq 75$)   & \\
    .. (B-4 $\leq 10$ \& B-S $\geq 70$)   & \\
    .. (B-4 $\leq 10$ \& B-S $\geq 65$)   & \\
    \bottomrule
\end{tabular}}
\caption{Performance of T5 model fintetuned on several Multipit data setups. Models are evaluated on the Multipit test set.}
\label{table:generation_setup_comparison}
\end{table*}
